# Supplementary material for: What if Eye...? Computationally Recreating Vision Evolution
Source: arXiv:2501.15001 source file (2025-02-13)
Supplement: Supplementary file 1 [file appendix_standalone.tex]

\documentclass[class=article, crop=false]{standalone}

\usepackage{graphicx}%
\usepackage{multirow}%
\usepackage{amsmath,amssymb,amsfonts}%
\usepackage{amsthm}%
\usepackage{mathrsfs}%
\usepackage[dvipsnames]{xcolor}%
\usepackage{textcomp}%
\usepackage{manyfoot}%
\usepackage{subcaption}%
\usepackage{booktabs}%
\usepackage{algorithm}%
\usepackage{algorithmicx}%
\usepackage{algpseudocode}%
\usepackage{listings}%
\usepackage{ifthen}%
\usepackage{lmodern}%
\usepackage{anyfontsize}%
\usepackage{xspace}%

\usepackage{cleveref}%

\input{macros}

\begin{document}
% \begin{appendices}

\input{sections/appendix/appendix_design_space}
\input{sections/appendix/appendix_optimizers}

\bibliography{sn-bibliography}% common bib file
% \end{appendices}

\end{document}
